# Supplementary material for: Adaptive Boosting for Domain Adaptation: Towards Robust Predictions in Scene Segmentation
Source: arXiv:2103.15685 source file (2022-09-22)
Supplement: Supplementary file 1 [file appendix.pdf]

# Adaptive Boosting for Domain Adaptation: Towards Robust Predictions in Scene Segmentation

## SUPPLEMENTARY MATERIAL

### A. Further Analysis and Discussions

**Network Structure.** We also verify the proposed method on a relatively vanilla network, *i.e.*, VGG16 [3]. Following previous works, we do not introduce BN (Batch Normalization) layers in the backbone network. We re-implement the MRNet [7], which has achieved 25.5% mIoU on GTA5  $\rightarrow$  Cityscapes. As shown in Table 6, we can observe two main points. First, the proposed method is complementary to the existing works, *e.g.*, MRNet [7], and the MRNet [7] + Ours achieves +14.0% mIoU improvements. Second, we also achieve one competitive result 39.5% mIoU with other existing methods based on VGG16.

| Method                 | Backbone | mIoU |
|------------------------|----------|------|
| Curriculum DA [6]      | VGG16    | 28.9 |
| Wang <i>et al.</i> [5] | VGG19    | 33.1 |
| CyCADA [2]             | VGG16    | 35.4 |
| CBST-SP [8]            | VGG16    | 36.1 |
| MRNet* [7]             | VGG16    | 25.5 |
| MRNet* [7] + Our       | VGG16    | 39.5 |

Table 6. Ablation Study on the effectiveness of the proposed method on a relatively vanilla network, *i.e.*, VGG16 [3] on GTA5  $\rightarrow$  Cityscapes. \*: We re-implement MRNet [7].

**vs. Mean Teacher (MT).** Similarly, the existing method, *i.e.*, Mean Teacher (MT) [4] also preserves one weight-average model during the training process. The main difference between the proposed method and Mean Teacher (MT) are two points: First, we adopt the adaptive sampler, which enables interactions between learned models and the data sampler. In this way, the proposed method leads to more complementary snapshots during training for the student aggregation. Second, Mean Teacher demands extra model inference to calculate the kl-divergence loss (costs extra time and memory), and forces the student model and the weight-average teacher model to predict the same distribution given the input, which also limits learning complementary student models. In contrast, the proposed method does not introduce such an objective and performs more efficiently and effectively with the spirit of AdaBoost [1]. As a result, the proposed method outperforms MT(Student) 46.6% and MT(Teacher) 47.5% mIoU (see Table 7).

| Method                   | mIoU |
|--------------------------|------|
| MRNet [7]                | 45.5 |
| MRNet [7] + MT (Student) | 46.6 |
| MRNet [7] + MT (Teacher) | 47.5 |
| MRNet [7] + Our          | 49.0 |

Table 7. Comparison with Mean Teacher (MT) [4].

### References

- [1] Yoav Freund, Robert E Schapire, et al. Experiments with a new boosting algorithm. In *ICML*, 1996.
- [2] Judy Hoffman, Eric Tzeng, Taesung Park, Jun-Yan Zhu, Phillip Isola, Kate Saenko, Alexei A Efros, and Trevor Darrell. Cycada: Cycle-consistent adversarial domain adaptation. In *ICML*, 2018.
- [3] Karen Simonyan and Andrew Zisserman. Very deep convolutional networks for large-scale image recognition. *arXiv:1409.1556*, 2014.

- [4] Antti Tarvainen and Harri Valpola. Mean teachers are better role models: Weight-averaged consistency targets improve semi-supervised deep learning results. In *NeurIPS*, 2017.
- [5] Qi Wang, Junyu Gao, and Xuelong Li. Weakly supervised adversarial domain adaptation for semantic segmentation in urban scenes. *IEEE Transactions on Image Processing*, 28(9):4376–4386, 2019.
- [6] Yang Zhang, Philip David, and Boqing Gong. Curriculum domain adaptation for semantic segmentation of urban scenes. In *ICCV*, 2017.
- [7] Zhedong Zheng and Yi Yang. Unsupervised scene adaptation with memory regularization in vivo. In *IJCAI*, 2020.
- [8] Yang Zou, Zhiding Yu, BVK Vijaya Kumar, and Jinsong Wang. Unsupervised domain adaptation for semantic segmentation via class-balanced self-training. In *ECCV*, 2018.
